# Supplementary material for: Plasmonic nanoantenna design and fabrication based on evolutionary optimization
Source: arXiv:1511.05438 ancillary file (2016-01-31)
Supplement: Supplementary file 1 [file 15_1116_Exp_EA_suppl_final.pdf]

# Plasmonic nanoantenna design and fabrication based on evolutionary optimization Supplementary Information

Thorsten Feichtner,[*,†,‡] Oleg Selig,[†,¶] and Bert Hecht[*,†]

*Nano-Optics & Biophotonics Group, Department of Experimental Physics 5, Röntgen Research Center for Complex Material Research (RCCM), Physics Institute, University of Würzburg, Am Hubland, D-97074 Würzburg, Germany*

E-mail: thorsten.feichtner@helmholtz-berlin.de.de; bert.hecht@physik.uni-wuerzburg.de

## FIB benchmarking

In order to determine geometrical restrictions of structures that are fabricated by focused ion beam milling, an 11×11 matrix test pattern was developed (see Fig. S1 left). The test pattern includes all relevant structural primitives, such as e.g. isolated gold islands, individual missing pixels (holes) and solid gold rims and corners.

Figure S1 right shows an SEM picture of the structure with the final reproducible dimensions by means of FIB-milling. The holes have a diameter of 22 nm and their center-to-center distance is 30 nm.

[*]To whom correspondence should be addressed

[†]Nano-Optics & Biophotonics Group, Department of Experimental Physics 5, Röntgen Research Center for Complex Material Research (RCCM), Physics Institute, University of Würzburg, Am Hubland, D-97074 Würzburg, Germany

[‡]Max-Plank-Institute for the Science of light, Günther-Scharowsky-Str. 1; Bldg. 24; D-91058 Erlangen

[¶]FOM Institute AMOLF, Biomolecular Photonics Group, Science Park 104, 1098 XG Amsterdam, The Netherlands

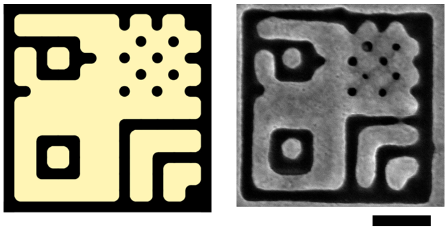

Figure S1: 11×11 test pattern design for FIB benchmarking. Left: Sketch of geometry. Right: SEM picture of the resulting structure produced by FIB milling in 30 nm thick monocrystalline gold (scale bar = 100 nm).

# Details of the evolutionary algorithm

One run of the evolutionary algorithm consists of consecutive generations containing 30 individuals each as depicted in the upper panel of Fig. S2. In the initialization step the very first generation $g = 1$ is built randomly, but with a given filling factor here $p_{\text{fill}} = 0.7$. This value has proven beneficial for high fitness optical antennas. All subsequent generations $g > 1$ are built from the best eight individuals of the preceding generation $g-1$, their fitness being evaluated via FDTD simulations. Each new individual is generated via mutation with a probability of 0.4 or crossing with a probability of 0.6 (see Fig. S2 bottom). Mutation happens by switching each bit of the binary genome with a probability $p_{\text{fl}} = 0.01$, resulting in an average of $\sum_{i=0}^{n} p_{\text{fl}}(1-p_{\text{fl}})^i = 0.7$ flips for $n = 120$ matrix elements ($11^2 - 1$; center spot is always free). Crossing mixes the genomes of two parents to generate a child. This mixing is realized in two different ways with equal probability, called 'linear' and 'spiral'. In the linear case the left part of an antenna $A$ (painted blue in Fig. S2)up to a random matrix element is used and complemented with the right part of another antenna $B$ (painted green). In the spiral case the inner part of an antenna $A$ was complemented with the outer part of antenna $B$, and the size of the inner part was also determined randomly. A more detailed description together with a graphical explanation can be found in.[1]

The development of the fitness parameter within the present evolutionary algorithm as a function of the simulation number and the generation number is plotted in Fig. S3. The mean and maximal fitness per generation do not increase monotonically since the algorithm

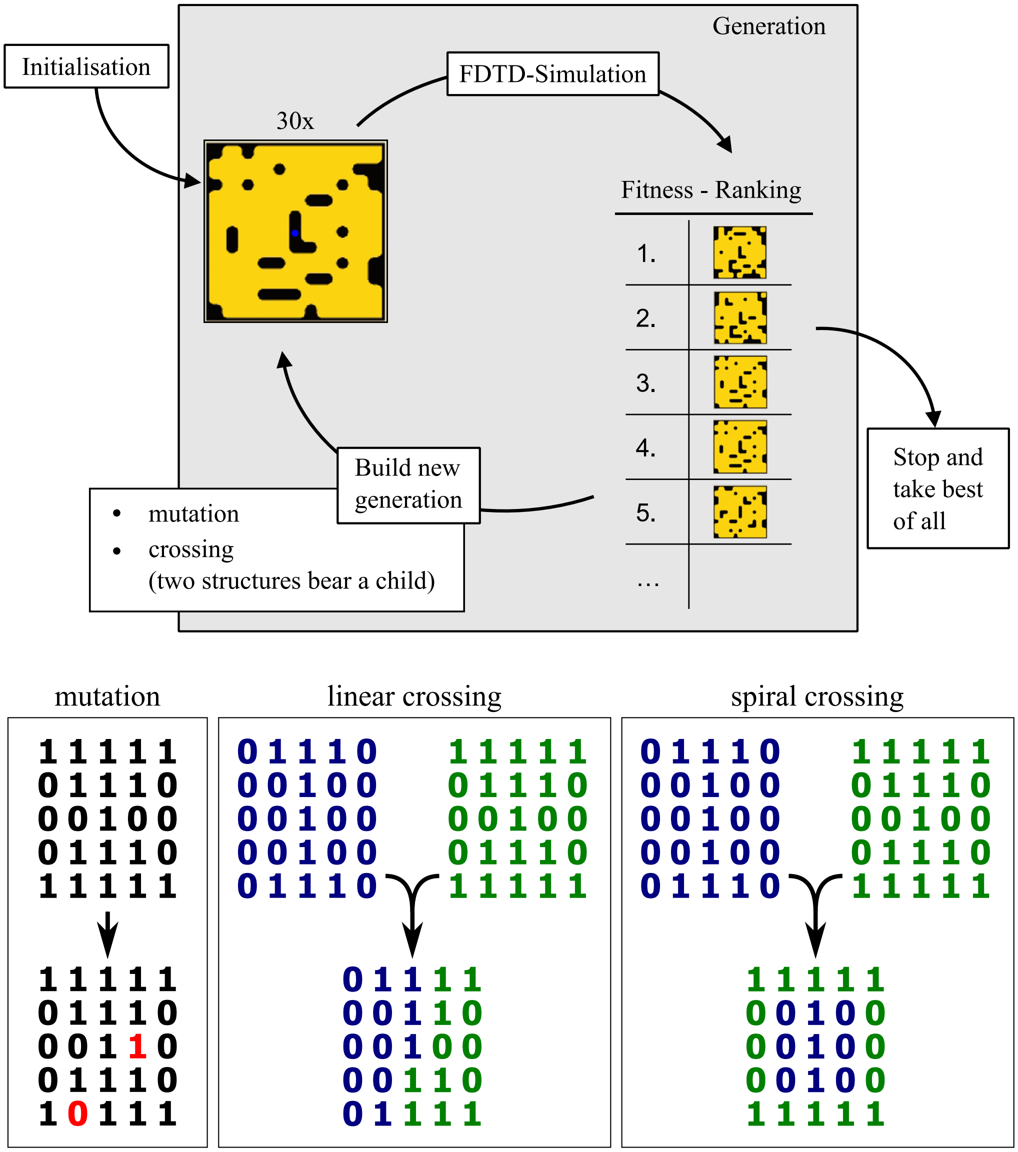


Figure S2: Working principle of the evolutionary algorithm. Upper panel: Flowchart of the EA steps. Initially the fitness parameter of 30 random structures is evaluated by means of FDTD simulations. After ranking, the best eight are used for building the next generation by means of mutation and crossing. Bottom panel: Methods of inheritance. Left: Mutation changes single bits (red) with a given probability. Linear and spiral crossing mix the genome of two different parents (blue and green). Linear crossing combines left and right parts, while spiral crossing combines inner and outer parts of two parents.

avoids evaluations of redundant geometries. If a reproduction mechanism yields a already evaluated structure (or an mirrored, physically identical version of an already evaluated structure), it will be omitted and the reproduction will be repeated. Mutation introduces eventually new geometries into the gene pool of the EA and the algorithm is able to escape local fitness maxima in configuration space leading to a temporary reduction of the maximal fitness followed by an increase in fitness in later generations.

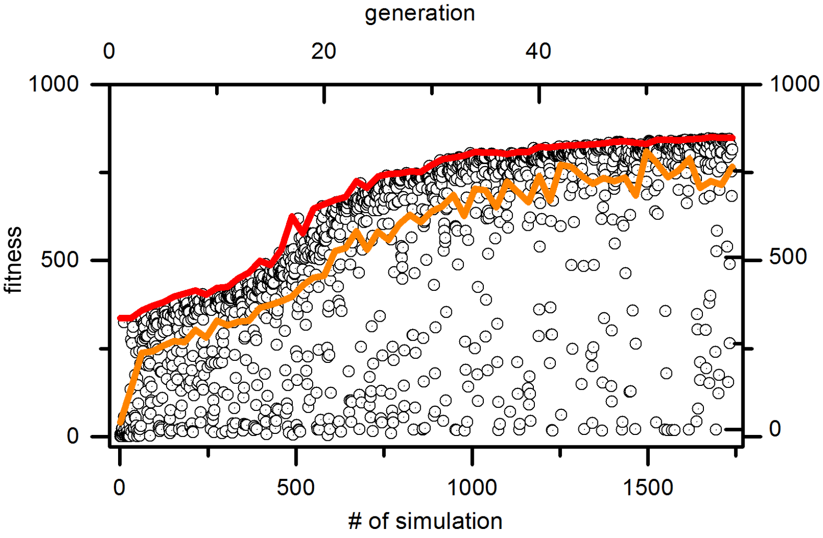


Figure S3: Development of the fitness parameter for the EA discussed here. Each point denotes a single individual. Also the best fitness per generation (red) as well as the mean fitness per generation (orange) are shown.

# AFM measurement of antenna thickness

The actual thickness of the fabricated structures has been measured by means of AFM (see Fig. S4). The pristine flake has a thickness of $48 \pm 1$ nm (area marked green) and the homogeneously ablated area, so-called polished area is reduced in height by $20 \pm 1$ nm (area marked blue). This results in a measured optical antenna thickness of $28 \pm 2$ nm, which is slightly less than the intended 30 nm.

The measurement was performed under ambient conditions using a tapping mode AFM operating at a resonance frequency of $240 - 280$ kHz and a scanning rate of 0.2 Hz (DMLS

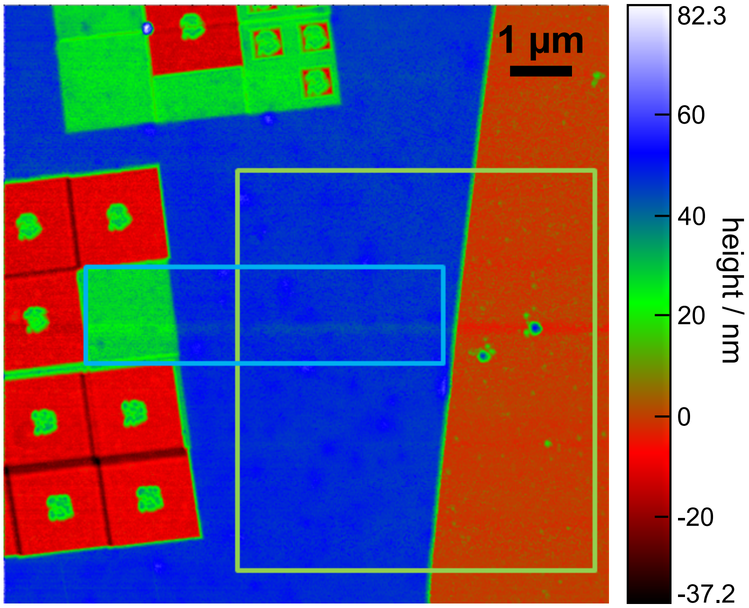


Figure S4: AFM measurement used for the determination of optical antenna thickness. The green and blue marked areas were used to evaluate height histograms.

scanning head, Nanoscope IIIa, Digital Instruments).

## Influence of reduced antenna height on the antenna resonance

To assess the effect of a decreased thickness on the fitness of the evolutionary antennas, simulations of the six fabricated geometries were performed and the results plotted in Fig. S5. The fitness is reduced for thinner antennas, as the resonance shifts into the red,[2] away from the wavelength of optimization. Except for antenna #5 the fitness hierarchy is maintained which van be explained with the spectra of all antennas (Figure S7). Antenna #5 is the only one with a relative blue shift with respect to the optimization wavelength, therefore being the only antenna optimized by the red shift.

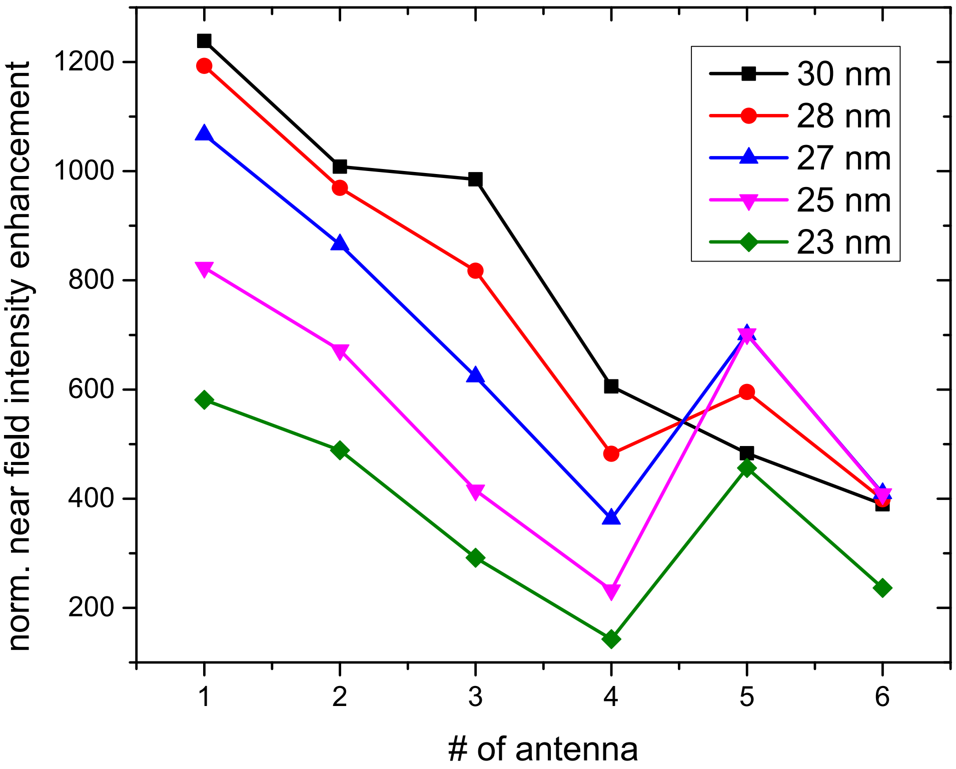

Figure S5: Change in fitness of evolutionary antennas for different layer thicknesses. The best four antennas decrease in near-field intensity enhancement as their thickness is reduced, the last two behave not systematically.

## Influence of hole diameter on the antenna resonance

The fabrication of the holes and lines needed to realize the evolutionary antennas has a uncertainty of ±1 nm. The influence of such a deviation in the geometry on the fitness all six fabricated antennas has been simulated by increasing as well as decreasing all hole diameters by 1 nm. The results in Fig. S6 show nearly no influence of this parameter on the relative fitness hierarchy. The large absolute fitness increase for smaller hole sizes – which is about 100 $nm^{-1}$ – originates from the enhanced capacitive coupling in the center gap, when the accumulating charges are less separated. This observation also explains the error bar within the TPPL measurements for all structures.

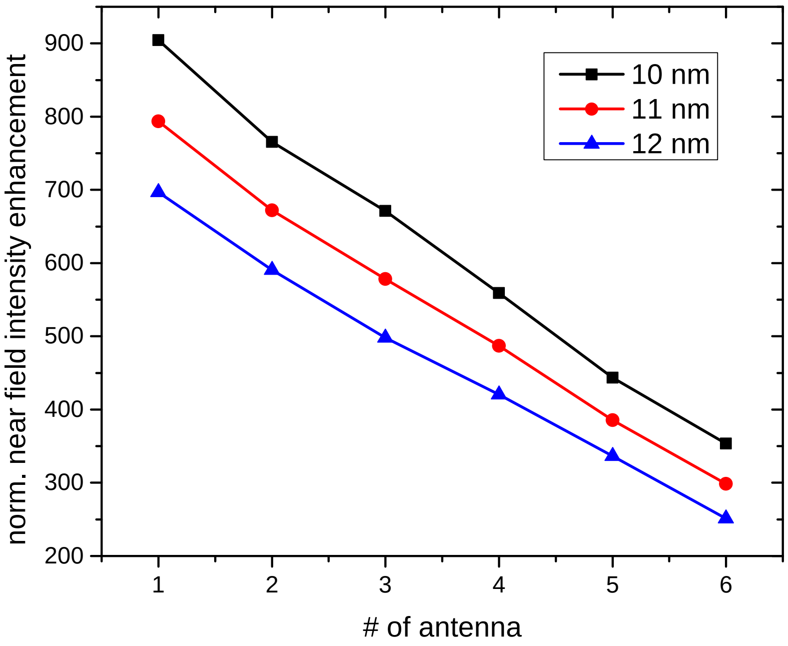


Figure S6: Change in fitness of evolutionary antennas dependent on the hole diameter / line width. As the width gets smaller, the near-field intensity enhancement increases by a large margin.

## Broadband spectra of EA antennas

To understand the experimental results it is necessary to know the broadband spectrum of the antennas. While the simulations within the EA are only taking the concentration of incoming far-field radiation into account, in the experiment the TPPL emission into the far-field also depends on the antenna spectrum at lower wavelengths, possibly leading to an enhancement and shaping of the TPPL signal.[3]

Figure S7 shows the simulated near field intensity enhancement spectra of the six fabricated antennas in a range of 500 - 900 nm recorded in the very center of the structure. Antennas #5 and #6 are the only structures showing a small peak at about 700 nm, potentially leading to an increased TPPL emission in the detection wavelength range (500 - 700 nm).

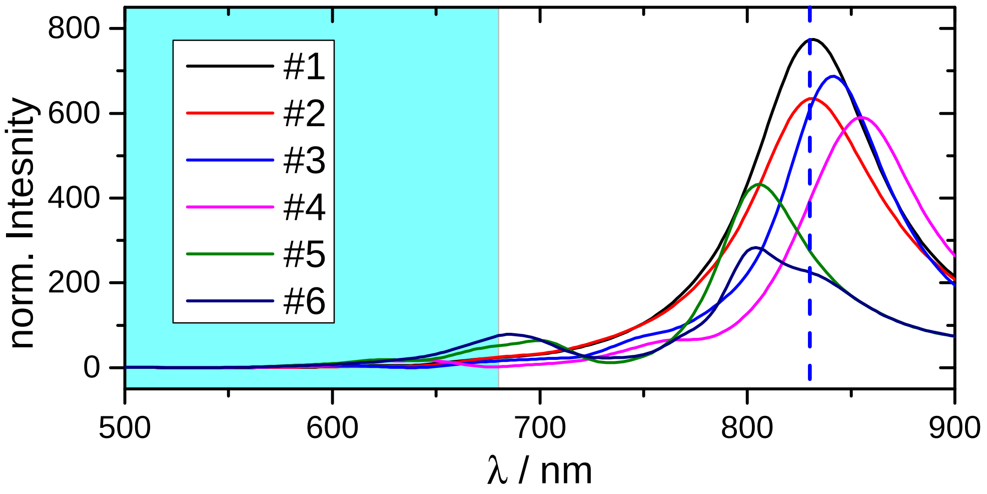


Figure S7: Near field spectra of the evolutionary antennas. The dark blue dashed line denotes the excitation wavelength of 830 nm, while the light blue area shows the wavelengths contributing to the TPPL signal in the experiment.

## Experimental setup

The optical setup is a home-built confocal microscope (see Fig. S8). The antennas where excited using a pulsed laser at a center wavelength of $\lambda$ = 830 nm (pulse length 300 fs,

repetition rate 76 MHz, Coherent Inc. MIRA 900) focused via an oil immersion objective (Nikon, Plan APO 100x, NA=1.4). The detection path - separated by a non-polarizing 50:50 cube beam splitter - three filters (notch filter: OD > 6 bei 830nm, Kaiser Optical System; two short pass filters: SP785 and SP680, Semrock) ensured the blocking of the direct reflection of the excitation laser and the detection of wavelengths. The signal was focused onto a single photon counting module (PDM Series, Micro Photon Devices).

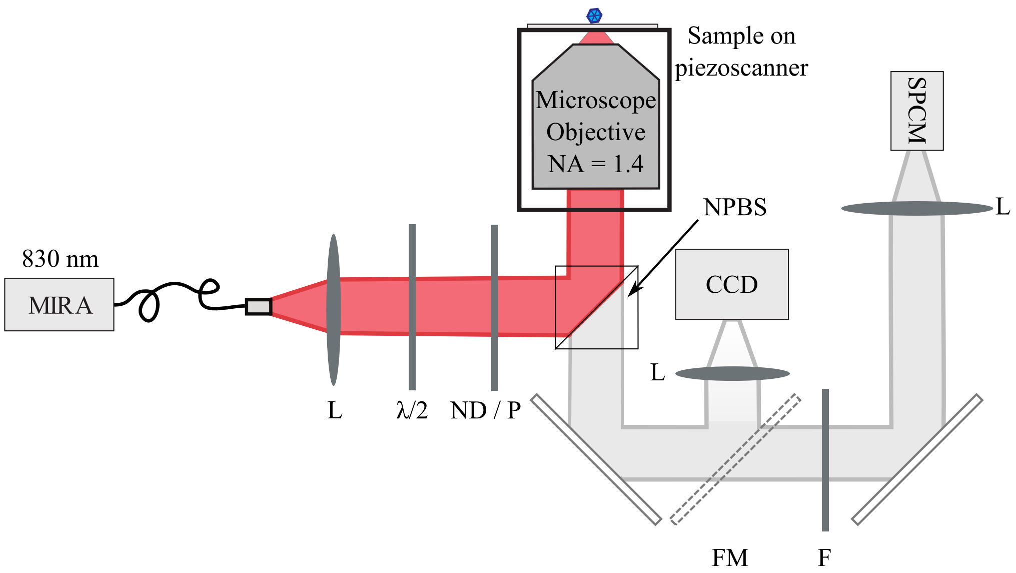


Figure S8: Experimental setup for TPPL microscopy. L: lens; ND/P: neutral density filter and polarizer; NPBS: non-polarizing beam-splitter; F: filters; FM: flip mirror. For further information see text.

## References


1. Feichtner, T.; Selig, O.; Kiunke, M.; Hecht, B. Evolutionary optimization of optical antennas. *Physical review letters* **2012**, *109*, 127701.

2. Biagioni, P.; Huang, J.-S.; Hecht, B. Nanoantennas for visible and infrared radiation. *Rep. Prog. Phys.* **2012**, *75*, 024402.

3. Wissert, M. D.; Ilin, K. S.; Siegel, M.; Lemmer, U.; Eisler, H.-J. Coupled nanoantenna

plasmon resonance spectra from two-photon laser excitation. *Nano letters* **2010**, *10*, 4161–5.
